# Supplementary material for: Single-beam grating-chip 3D and 1D optical lattices
Source: arXiv:2405.21065 ancillary file (2024-11-20)
Supplement: Supplementary file 1 [file Lattice_GMOT_Supplemental.pdf]

# Single-beam grating-chip 3D and 1D optical lattices - Supplementary Material

Alan Bregazzi,<sup>1</sup> James P. McGilligan,<sup>1</sup> Paul F. Griffin,<sup>1</sup> Erling Riis,<sup>1</sup> and Aidan S. Arnold<sup>1</sup>

<sup>1</sup>*SUPA and Department of Physics, University of Strathclyde, G4 0NG, Glasgow, United Kingdom*

## LATTICE MODEL AND DATA

The lattice input beam has a Gaussian electric field  $E_{\text{in}} = E_0 \exp(-(x^2 + y^2)/w^2) \exp(i\mathbf{k}_{\text{in}} \cdot \mathbf{r})$ , with a field  $E_0 = \sqrt{\frac{2I_0}{\epsilon_0 c}}$  for a beam of intensity  $I_0 = \sqrt{\frac{2P}{\pi w^2}}$  from a laser with power  $P$  and waist ( $1/e^2$  radius)  $w$ , wavenumber  $\mathbf{k}_{\text{in}} = \{0, 0, -k\}$  for  $k = 2\pi/\lambda$  and  $\mathbf{r} = \{x, y, z\}$ .

There are three ( $m \in \{-1, 0, 1\}$ ) sector-shaped diffracted orders from each of the three grating sectors ( $n \in \{0, 1, 2\}$ ), with associated k-vectors

$$\mathbf{k}_{m,n} = k\{-\sin(n\phi)\sin(m\theta), \cos(n\phi)\sin(m\theta), \cos(m\theta)\},$$

where  $\phi = 2\pi/N$  is the relevant rotation angle between the  $N = 3$  gratings, and  $\theta = \arcsin(\lambda/d)$  is the first order diffraction angle from a period  $d$  grating. The corresponding peak squareroot intensities are  $E_{m,n} = \sqrt{\eta_m \sec(m\theta)} E_0$ , which allows for grating order diffraction efficiencies  $\eta_m$ , and intensity increases  $\sec(m\theta)$  in diffracted beams due to geometrical compression [1].

The total field is determined by summing the phase-shifted field amplitudes from the input beam and all diffracted orders. To determine the lattice depths, frequencies and scattering rates, we use a very similar formalism to that in Ref. [2]. Note the estimated 3D lattice

frequencies are overestimates, as due to the other current uncertainties we have used a simple scalar electric field superposition instead of incorporating the full 3D laser polarisations.

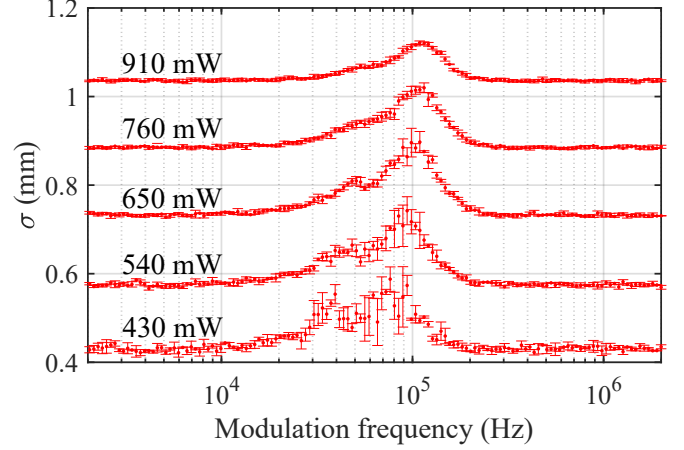

FIG. A2. Experimental spectra of 3D lattice vibrational heating, with detuning  $\Delta = -78$  GHz and beam powers of Fig. 2a, i.e.: (430, 540, 650, 760, 910) mW. Each dataset is vertically offset by 0.15 mm.

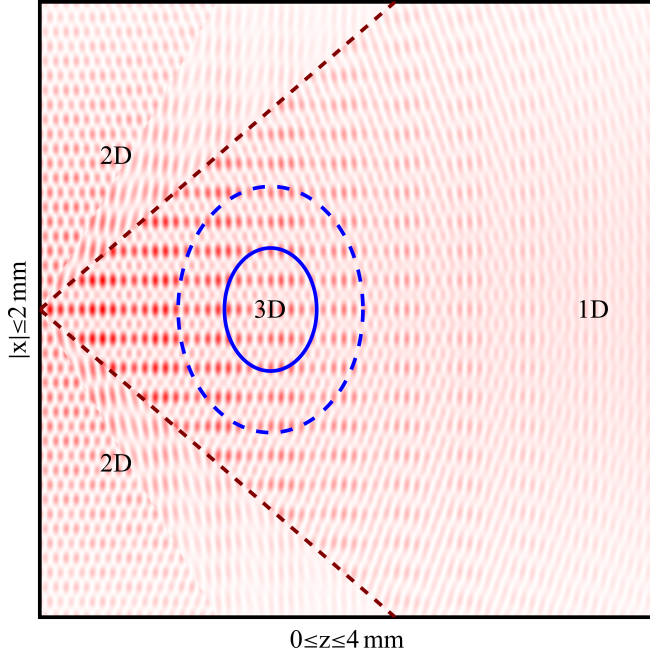

FIG. A1. The 3D lattice light intensity (red linear shading) is indicated in the  $4 \times 4 \text{ mm}^2$   $zx$ -plane at  $y = 0 \text{ mm}$  – the final slice through the MOT, orthogonal to both Fig. 1 a and b.

## IMAGING

In order to explain the atomic motion after time-of-flight in Fig. 1 d. We consider the maximum initial standard deviation of ‘hot’ atoms filling the 1D lattice of  $\sigma_y = 40 \mu\text{m}$  due to the  $80 \mu\text{m}$  beam waist. One millisecond of free expansion followed by  $150 \mu\text{s}$  of highly saturated resonant fluorescent scattering during imaging should heat the atoms from  $\approx 10 \mu\text{K}$  to  $700 \mu\text{K}$  but only spread the cloud to  $\sigma_y = 44 \mu\text{m}$ . The largest change, however, is due to reradiation forces from the resonant light in the dense atom cloud [3], acting mainly in the direction of density gradients. As the sub-micron scale lattice density modulation in the  $z$  direction is very short-lived, this force is basically radial. Using estimates based on Ref. [3], we find acceleration at the start of resonant imaging around  $a = 10^4 \text{ m/s}^2$ . Within a factor of two, this acceleration leads to an expansion which quantitatively matches the observed cloud width of  $\sigma_y = 118 \mu\text{m}$  seen in Fig. 1 d.

- 
- [1] M. Vangeleyn, P. F. Griffin, E. Riis, and A. S. Arnold, Laser cooling with a single laser beam and a planar diffractor, *Optics Letters* **35**, 3453 (2010).
- [2] V. A. Henderson, M. Y. H. Johnson, Y. B. Kale, P. F. Griffin, E. Riis, and A. S. Arnold, Optical characterisation of micro-fabricated Fresnel zone plates for atomic waveguides, *Optics Express* **28**, 9072 (2020).
- [3] A. S. Arnold and P. J. Manson, Atomic density and temperature distributions in magneto-optical traps, *Journal of the Optical Society of America B* **17**, 497 (2000).
